# Supplementary material for: Effects of ferroelectric polarization on surface phase diagram: an evolutionary algorithm study of the BaTiO$_{3}$(001) surface
Source: arXiv:1505.06830 source file (2015-05-26)
Supplement: Supplementary file 1 [file supp.pdf]

# Supplementary Material for "Effects of ferroelectric polarization on surface phase diagram: an evolutionary algorithm study of of the $BaTiO_3(001)$ surface"


Pengcheng Chen[1,2], Yong Xu[1,2,3], Na Wang[1,2], Artem R Oganov[5,6,7], Wenhui Duan[1,2,4*]

[1] *Department of Physics and State Key Laboratory of Low-Dimensional Quantum Physics, Tsinghua University, Beijing, 100084, People's Republic of China*

[2] *Collaborative Innovation Center of Quantum Matter, Tsinghua University, Beijing 100084, People's Republic of China*

[3] *Department of Physics, McCullough Building, Stanford University, Stanford, California 94305-4045, USA*

[4] *Institute for Advanced Study, Tsinghua University, Beijing 100084, Peoples Republic of China*

[5] *Department of Geosciences, Center for Materials by Design, and Institute for Advanced Computational Science, State University of New York, Stony Brook, NY 11794-2100*

[6] *Moscow Institute of Physics and Technology, Dolgoprudny city, Moscow Region, 141700, Russian Federation*

[7] *Northwestern Polytechnical University, Xi'an, 710072, China*



(Dated: May 13, 2015)


## I. Electronic Structure

In the ferroelectric thin film, the local bands are shifted by the electrostatic potential. When the accumulated electrostatic potential exceeds the energy gap of the bulk phase, a charge redistribution takes place, leading to the compensating surface charges and the surface metallization, as schematized in Fig. S1(a). Our calculated layer-projected density of states (DOS) of the $BaTiO_3$ slab without surface reconstruction [Fig. S1(b)] is consistent with this general picture. Due to the charge transfer, the ideal surface, either BaO- or $TiO_2$-terminated surface becomes metallic. The surface metallicity, more specifically, can be regarded as $n$ and $p$ types for the $\boldsymbol{P}_\uparrow$ and $\boldsymbol{P}_\downarrow$ conditions, respectively [Fig. S1(c)]. Compared to ideal $TiO_2$-terminated surface, the relatively lower density of states around the Fermi level indicate the weaker metallicity of ideal BaO-terminated surface.

To reveal the effects of surface reconstruction on the electrostatic stability, we have calculated the resulting spatial distribution of electrostatic potential, by taking the energy level of Ti $3s$ orbital in each bulk-like cells as the reference of the potential $\Phi$, as shown in Fig. S2. Neutral $TiO_2$-overlayer-type phases retain the features of the ideal $TiO_2$-terminated slab that the electrostatic potential keep increasing/decreasing from the bottom layer. In the $\boldsymbol{P}_\downarrow$ condition, the charge transfer [Fig. S3(b)] induced by the TiO adunit produces an electric field opposite to the depolarization field, strongly reducing the potential accumulation at the surface. However, in the $\boldsymbol{P}_\uparrow$ condition the scenario is different, the TiO-adunit induced electric field is along the direction of the depolarization field, enhancing the potential accumulation at the surface. The results of the calculated enhancement/reduction of the surface potential are in good agreement with the calculated relative surface energies.

Fig. S4 shows the calculated surface DOS of the stable phases, $(2\times1)$-TiO and $(1\times1)$-$TiO_2$ in the different polarization conditions. For the $(1\times1)$-$TiO_2$ cases, the electronic structure of the surface remains almost unchanged compared to the ideal $TiO_2$-terminated surface. For the $(2\times1)$-TiO case in the $\boldsymbol{P}_\downarrow$ condition, along with the strong reduction of the electrostatic potential accumulation and charge transfer effect, the significant change in the surface electronic structure can be found, i.e., from the $p$-type metallicity to the $n$-type metallicity.

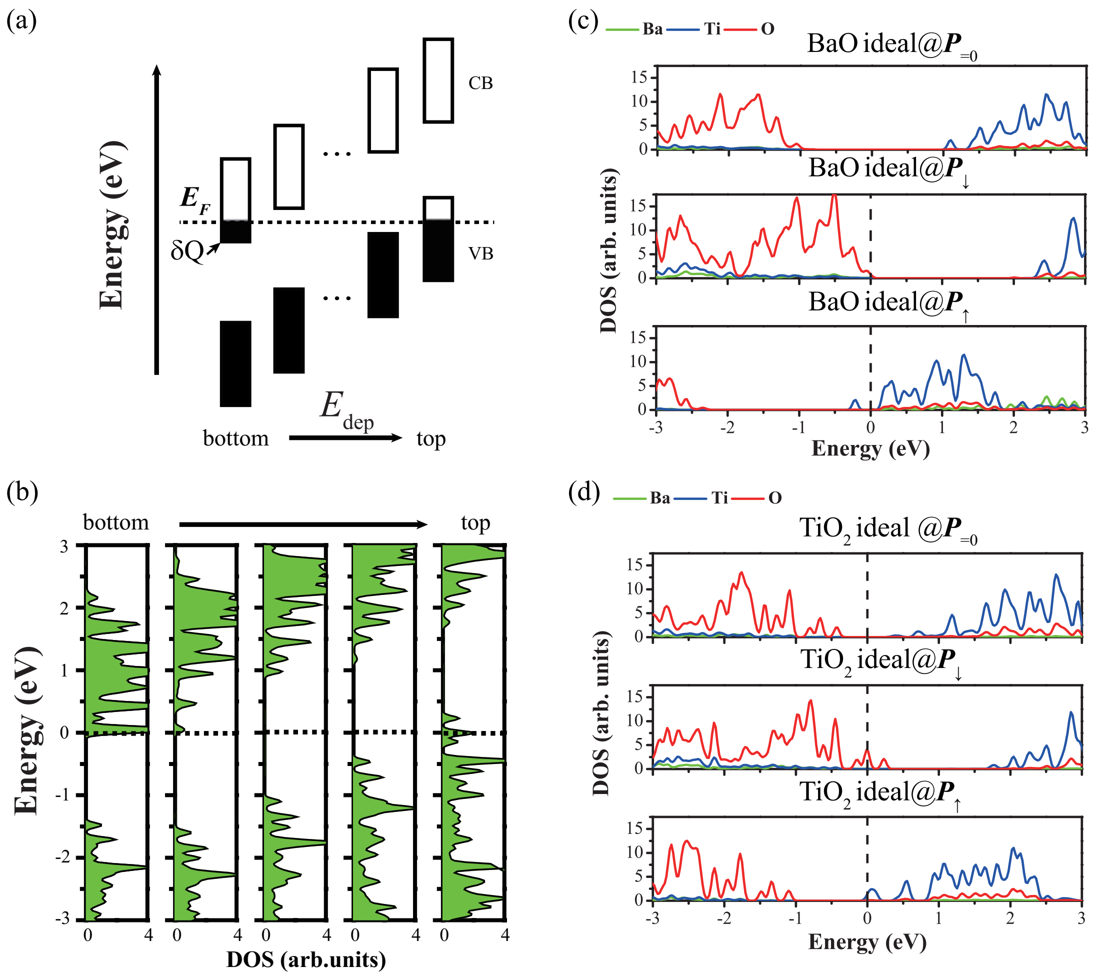


FIG. S1: (Color online) (a) Schematic of the electronic structure of ferroelectric thin film. The overall gap is closed due to electrostatic potential accumulation by the depolarization field. Here $\delta Q$ denotes the charge transfer from the top layer to the bottom layer. (b) Calculated layer resolved density of states (DOS) of ideal $TiO_2$-terminated $BaTiO_3$ slab in the $\boldsymbol{P}_{\downarrow}$ condition. (c)/(d) Calculated surface DOS of ideal BaO-/$TiO_2$-terminated $BaTiO_3$ slab in different polarization conditions. The Fermi level is set at zero.

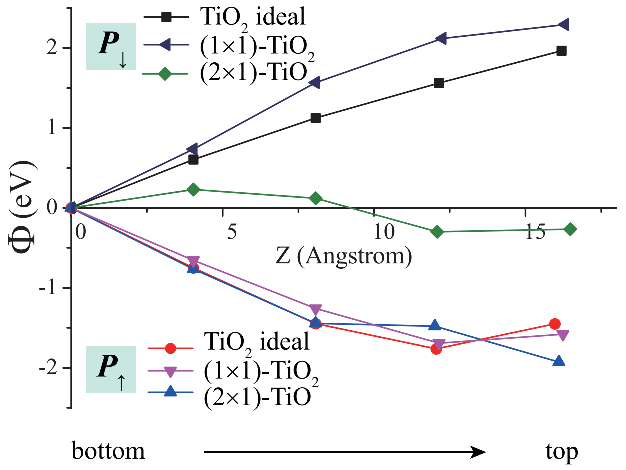


FIG. S2: (Color online) The relative electrostatic potential $\Phi$ of $BaTiO_3$ slabs with different surface configurations. The $\Phi$ of the bottom layer of the slab is taken as the reference zero.

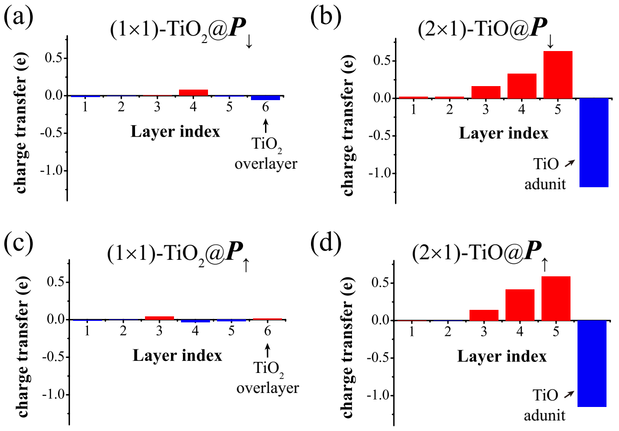


FIG. S3: (Color online) Calculated layer-resolved charge transfer of $BaTiO_3$ slabs with different surface configurations (red and blue represent electron accumulation and depletion, respectively).

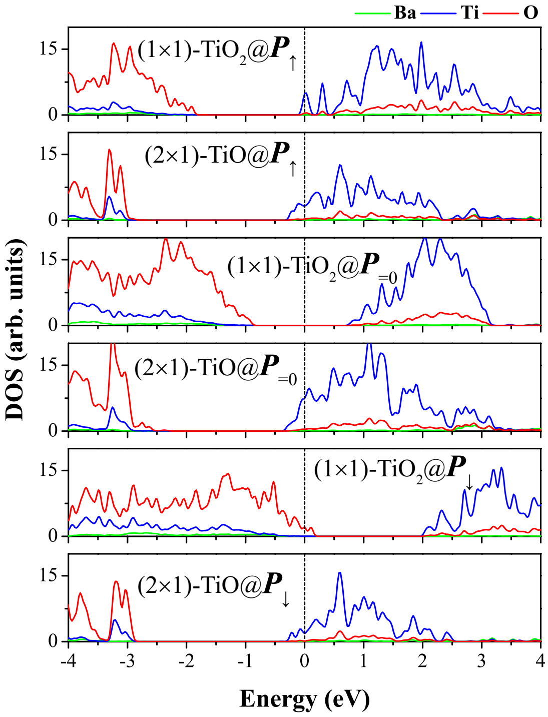


FIG. S4: (Color online) Calculated surface DOS of representative phases, i.e., (2×1)-TiO and (1×1)-$TiO_2$, in the different polarization conditions. Ti-, Ba- and O-resolved DOS are shown in blue, green and red lines, respectively.

## II. The temperature effect

Following the approach of Reuter and Scheffler[1], the temperature-dependent Gibbs free energy of the slab is approximated by the sum of DFT total energy at zero temperature and the vibration energy at finite temperature, neglecting the $pV$ term($\sim 10^{-3}$ meV/Å$^2$). In turn, the Gibbs free energy of the slab is written as

$$G_{\text{slab}} = E^{\text{DFT}}(\text{slab}) + F^{\text{VIB}}(\text{slab}). \tag{S1}$$

Generally the vibration energy contribution can be obtained within the harmonic approximation by calculating the phonon dispersion[2]. However, as the large amount of computation, it is difficult to calculate the phonon dispersion of the whole slab. Note that only the relative surface free energy is meaningful to the determination of the phase diagram. The principal difference of the slabs comes from the different surface adsorbates. In this regard, we can

approximate the vibration energy contribution using the Einstein model by calculating the vibration frequencies of the surface adsorbates of different surface structures. Then the vibration energy can be written as

$$F^{\mathrm{VIB}}(T,\omega)=\frac{\hbar\omega}{2}+kT\ln(1-e^{-\frac{\hbar\omega}{kT}}) \tag{S2}$$

where $T$ and $\omega$ represent, respectively, the temperature of the system and the characteristic vibration frequency for the phonon modes. We use the finite displacement method to calculate the vibration frequency. The force constant matrix $\mathbf{K}$ is generated by calculating the force $\mathbf{F}$ of the atoms with the finite atomic displacement $\mathbf{X}$ applied,

$$\mathbf{F}=\begin{vmatrix} K_{xx} & K_{xy} & K_{xz} \\ K_{yx} & K_{yy} & K_{yz} \\ K_{zx} & K_{zy} & K_{zz} \end{vmatrix}\mathbf{X} \tag{S3}$$

and the vibration frequency is

$$\omega_i=\sqrt{\frac{K_i}{m_{\mathrm{atom}}}} \tag{S4}$$

where $i$ represents the vibration mode, $K_i$ is the $i$-th eigenvalue of the force constant matrix, and $m_{\mathrm{atom}}$ is the atomic mass. Table S1 just lists the calculated average characteristic vibration frequency and the total vibrational free energy at 1100 K of surface absorbates of different stable phases involved in the 0 K phase diagram.

Due to the requirement for the surface to be in equilibrium with the bulk barium titanate and to keep barium, titanium and oxygen atoms from precipitating on the surface, the accessible chemical potential boundary conditions go to,

$$\mu_{\mathrm{Ba}}+\mu_{\mathrm{Ti}}+3\mu_{\mathrm{O}}=g^{\mathrm{Bulk}}_{\mathrm{BaTiO_3}}(T,p) \tag{S5}$$

$$\mu_{\mathrm{Ba}}\le g^{\mathrm{Bulk}}_{\mathrm{Ba}}(T,p) \tag{S6}$$

$$\mu_{\mathrm{Ti}}\le g^{\mathrm{Bulk}}_{\mathrm{Ti}}(T,p) \tag{S7}$$

$$\mu_{\mathrm{Ba}}+\mu_{\mathrm{O}}\le g^{\mathrm{Bulk}}_{\mathrm{BaO}}(T,p) \tag{S8}$$

$$\mu_{\mathrm{Ti}}+2\mu_{\mathrm{O}}\le g^{\mathrm{Bulk}}_{\mathrm{TiO_2}}(T,p) \tag{S9}$$

where $g^{\mathrm{Bulk}}(T,p)$ is the Gibbs free energy of corresponding compounds. For solid phase compounds, temperature dependent $g^{\mathrm{Bulk}}(T,p)$ can be approximated with the sum of 0 K total energy ($E^{\mathrm{DFT}}_{\mathrm{Bulk}}$) obtained from DFT calculation and vibrational energy ($F^{\mathrm{VIB}}_{\mathrm{Bulk}}$(T,p)) at finite temperature computed within the harmonic approximation, using the PHONOPY package[2]. An energy correction has been applied to the $\mu_{\mathrm{O}}$ by taking the reference of experimental data of Gibbs free energy of formation of $BaTiO_3$, BaO and $TiO_2$[3–5]. The calculated data are listed in Table S2.

Fig. S5 shows the surface phase diagram at 1100 K with the vibration contribution included. Compared to the phase diagram in Fig. 2(a) at zero temperature, the accessible chemical potential boundaries are slightly shifted. However, the thermodynamically stable phase is still $(2\times1)$-TiO and the overall pattern of the calculated phase diagram does not change upon adding the vibration contribution. This shows that the temperature effect is negligible in the present case.

---

* Electronic address: `dwh@phys.tsinghua.edu.cn`

[1] K. Reuter and M. Scheffler, Physical Review B **65**, 035406 (2001).
[2] A. Togo, F. Oba, and I. Tanaka, Physical Review B **78**, 134106 (2008).
[3] K. Johnston, M. R. Castell, A. T. Paxton, and M. W. Finnis, Physical Review B **70**, 085415 (2004).
[4] J. A. Dean, *Lange's Handbook of Chemistry, 12th ed* (McGraw-Hill Book Company, New York, NY, 1979).
[5] M. Binnewies and E. Milke, *Thermochemical Data of Elements and Compounds* (Wiley-VCH Verlag GmbH, 2008), ISBN 9783527618347, URL `http://dx.doi.org/10.1002/9783527618347.ch5a`.

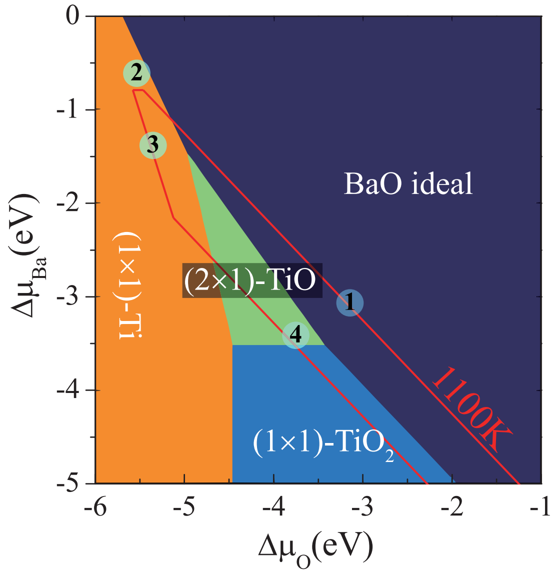


FIG. S5: (Color online) Surface phase diagram of $BaTiO_3(001)$ for $(1\times1)$ and $(2\times1)$ reconstructions in the $\mathbf{P}_{\downarrow}$ condition. The vibration contribution is included. The red solid lines bound the chemical stability ranges of $BaTiO_3$. The precipitation lines of bulk BaO, Ba, Ti and $TiO_2$ are labeled as 1-4, respectively, which bound the accessible chemical potential range defined by thermal equilibria at 1100 K.

TABLE S1: Calculated average characteristic vibration frequency and total vibrational free energy at 1100 K of surface absorbates of different stable phases involved in the 0 K phase diagram.

| Phase | Atom | $\bar{w}$ ($cm^{-1}$) | $F^{vib}_{total}$ (1100 K) (eV) |
|---|---|---|---|
| $(2\times1)$-$Ti_2O_4$ | $Ti_1$ | 325 | -0.245 |
| | $Ti_2$ | 317 | -0.267 |
| | $O_1$ | 491 | -0.248 |
| | $O_2$ | 385 | -0.200 |
| | $O_3$ | 550 | -0.110 |
| | $O_4$ | 422 | -0.166 |
| $(1\times1)$-$TiO_2$ | $Ti_1$ | 336 | -0.236 |
| | $O_1$ | 374 | -0.232 |
| | $O_2$ | 428 | -0.166 |
| $(2\times1)$-TiO | $Ti_1$ | 382 | -0.215 |
| | $O_1$ | 420 | -0.264 |
| $(2\times1)$-Ti | $Ti_1$ | 258 | -0.311 |
| $(1\times1)$-Ti | $Ti_1$ | 247 | -0.324 |
| | $Ti_2$ | 247 | -0.324 |
| $(2\times1)$-$Ti_2O$ | $Ti_1$ | 236 | -0.345 |
| | $Ti_2$ | 324 | -0.243 |
| | $O_1$ | 372 | -0.223 |
| BaO ideal | $Ba_1$ | 103 | -0.58 |
| | $O_1$ | 331 | -0.249 |

TABLE S2: Calculated and experimental Gibbs free energy of formation $\Delta_f G^0$ of various compounds (in units of eV).

| Compound | Cal. | Exp. |
|---|---|---|
| $BaTiO_3$(tetragonal) | -16.29 | -16.29[4] |
| $TiO_2$(anatase) | -9.79 | -9.25[5] |
| BaO | -5.25 | -5.36[5] |
